# Supplementary material for: mLUKE: The Power of Entity Representations in Multilingual Pretrained Language Models
Source: arXiv:2110.08151 source file (2022-03-30)
Supplement: Supplementary file 1 [file alignment.tex]

\section{Analyzing the Effect of Cross-lingual Representation Alignment by MEP}
\label{appendix:entity-alignment}

Wikipedia entity annotations have been used to provide rich cross-lingual alignment information to improve cross-lingual alignment of word representations \citep{Calixto2021naacl,XLM-K-2021-arxiv}.
However, unlike previous work, entity information is provided in the form of entity embeddings, which are separated from word embeddings, and thus it is unknown if the masked entity prediction (MEP) objective would affect the cross-lingual alignment of word representations.
In this section, we analyze the effect of alignment by comparing \mlukeW{} against \xlmr{}\extraTraining{}.
We show that MEP itself does not improve the alignment of output embeddings in both word-level and sentence-level, suggesting the improvement of \mlukeW{} in cross-lingual transfer QA \cref{sec:experiment-qa}, NER and RE \cref{sec:experiment-rc-ner} comes from entity-related knowledge learned in MEP.

\subsection{Analyzing Word-level Alignment}
We evaluate the alignment of word representations as performance on the contextualized word retrieval (CWR) task with the MLQA dev set \citep{lewis-etal-2020-mlqa} as in \cref{subsec:qa_analysis}.

Table \ref{table:squad_retrieval_appendix} shows the performance in terms of the mean reciprocal rank score.
We find that the scores of \mlukeW{} exhibit lower scores than \xlmr{}\extraTraining{}, which is trained with exactly the same amount of data as \mlukeW{}.
This shows that the masked entity prediction does not improve the alignment or output embeddings in word-level.

\begin{table}[ht]
%   \small
%   \setlength\tabcolsep{4pt}
  \centering
  \begin{tabular}{lccccccc} \toprule
        &     ar      &     de     &     es     &     hi     &     vi     &     zh     &    avg.    \\ \midrule
% mBERT   &     63.9    &    82.1    &    87.8    &    65.1    &    85.2    &    75.1    &    76.5    \\
% XLM-R   &     36.5    &    59.3    &    67.3    &    43.5    &    63.6    &    45.5    &    52.6    \\
\xlmr{}\extraTraining{}  & 58.5    &    76.1    &    79.9    &    62.8    &    76.0    &    60.0    &    68.9    \\
\mlukeW{}  &    55.6    &    66.1    &    68.4    &    60.4    &    69.7    &    56.1    &    62.7    \\
% mLUKE-E  &    56.9    &    68.1    &    70.4    &    61.5    &    71.2    &    60.0    &    64.7   \\
  \bottomrule
  \end{tabular}
  \caption{The mean reciprocal rank score of the CWR task with the MLQA dev set.}
  \label{table:squad_retrieval_appendix}
\end{table}
\vspace{-4mm}

\subsection{Analyzing Sentence-level Alignment}
We evaluate the alignment of sentence representations with the task of parallel sentence matching with the Tatoeba dataset \citep{artetxe-schwenk-2019-massively}, which supports 112 languages.
This task is, given a set of parallel sentences, to retrieve the correct target sentence for each query sentence.
Here, we evaluate the average of the output embeddings from the models and perform the retrieval with the cosine similarity scores of the embeddings.
For each language pair, we compute the retrieval accuracy of the forward direction, {\it i.e.,}, English to the target language.

\begin{figure*}[h]
\begin{center}
  \includegraphics[width=6cm]{data/tatoeba/mLUKE_vs_XLM-R_with_training.png}
  \caption{The accuracy scores of parallel sentence matching for each language pair in the Tatoeba dataset.}
  \label{fig:tatoeba}
\end{center}
\end{figure*}

\Figure{fig:tatoeba} shows the results of \mlukeW{} and \xlmr{}\extraTraining{} for each language pair in the dataset.
We observe that \mlukeW{} provides slightly worse performance for the task, showing that MEP does not have an effect to align output embeddings across languages in sentence-level.
