# Supplementary material for: mLUKE: The Power of Entity Representations in Multilingual Pretrained Language Models
Source: arXiv:2110.08151 source file (2022-03-30)
Supplement: Supplementary file 2 [file comparison_with_other_models.tex]

\section{Comparison with Other Pretrained Models}
\label{appendix:more_results}

We repeat the results of MLQA in \Table{table:results-qa-with-other-baselines} with the results of other multilingual pretrained models taken from their original papers.
ERNIE-M \citep{Ouyang2020ERNIEMEM} and InfoXLM \citep{chi-etal-2021-infoxlm} are trained with parallel corpora while XLM-K \citep{XLM-K-2021-arxiv} is trained only with monolingual corpora and thus is closer to our setting.
% We also provide the result from a larger model, \mlukeE{}\la{}, whose backbone is \xlmr{}\large{}, to compare with the model in \citet{Calixto2021naacl}.
Notice, that the results from other papers share the same pretrained model backbone but are not directly comparable to our results because the fine-tuning settings are different.

\begin{table*}[h]
  % \small
  % \setlength\tabcolsep{5pt}
   \centering
  \begin{tabular}{lcccccccc} \toprule
    MLQA  &   en & es & de & ar & hi & vi & zh & avg.  \\ \midrule
  \mbert{} & 79.1 & 65.9 & 58.6 & 48.6 & 44.8 & 58.5 & 58.1 & 59.1 \\
  \xlmr{} & 79.7 & 67.7 & 62.2 & 55.8 & 59.9 & 65.3 & 62.5 & 64.7  \\
  \extraTraining{} & 81.3 & 69.8 & 65.0 & 54.8 & 59.3 & 65.6 & 64.2 & 65.7  \\
  \mlukeW{} & 81.3 & 69.7 & 65.4 & 60.4 & 63.2 & 68.3 & 66.1 & 67.8  \\
  \mlukeE{} & 80.8 & 70.0 & 65.5 & 60.8 & 63.7 & 68.4 & 66.2 & 67.9  \\
  \midrule
  ERNIE-M \citep{Ouyang2020ERNIEMEM} & 81.6 & 70.9 & 65.8 & 61.8 & 65.4 & 70.0 & 65.6 & 68.7 \\
  InfoXLM \citep{chi-etal-2021-infoxlm} & 81.3 & 69.9 & 64.2 & 60.1 & 65.0 & 70.0 & 64.7 & 67.9 \\
  XLM-K \citep{XLM-K-2021-arxiv} & 80.8 & 69.2 & 63.8 & 60.0 & 65.3 & 70.1 & 63.8 & 67.7  \\
%   \midrule
%   \citet{Calixto2021naacl}              & - & - & - & - & - & - & - & 70.1 \\
%   \mlukeE{}\la{}  & 83.7 & 74.1 & 70.4 & 66.1 & 70.8 & 73.8 & 70.1 & 72.7 \\
  \bottomrule
  \end{tabular}

  \caption{Results on the MLQA dataset in the cross-lingual transfer settings.}
  \label{table:results-qa-with-other-baselines}
\end{table*}

% The models trained with parallel corpora achieve comparable or better scores (the average score of 67.9 in InfoXLM and 68.7 in ERNIE-M) than \mlukeE{} (67.9).
% This suggests that our model could see further improvement when pretrained with cross-lingual supervision from parallel corpora.
